# Supplementary material for: Memory functions of magnetic skyrmions
Source: arXiv:1501.07650 ancillary file (2015-01-30)

**Supplementary Informations**

**Memory functions of magnetic skyrmions**

W. Koshibae, Y. Kaneko, J. Iwasaki, M. Kawasaki, Y. Tokura and N. Nagaosa

## Movie 1

Numerical result of Sk writing by heat in the case of Fig.2.

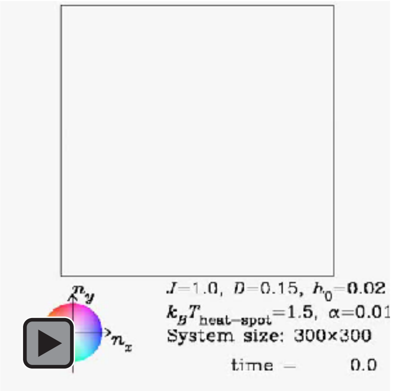


## Movie 2

Numerical result of Sk erasing by heat in the case of Fig.2.

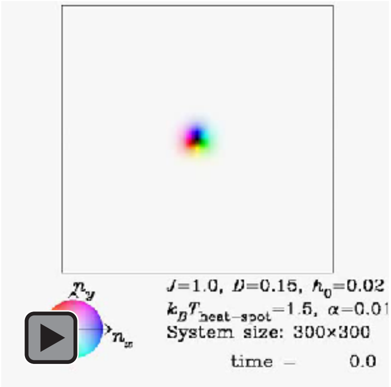


## Movie 3

Numerical result of Sk writing/erasing in the case of Fig.3.

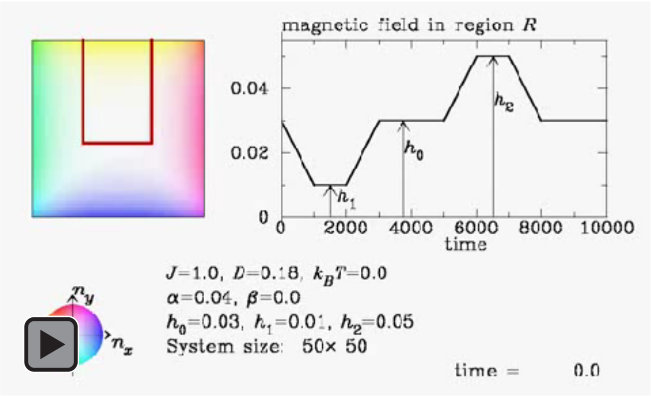

**Movie 4**

Numerical result of Sk writing/erasing in the case of Fig.4.

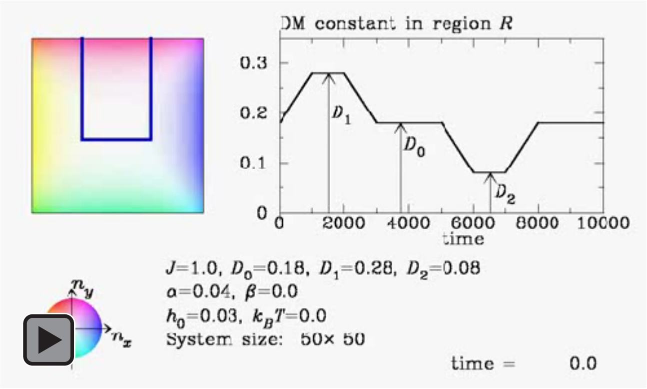


**Movie 5**

Numerical result of Sk writing/erasing in the case of Fig.5.

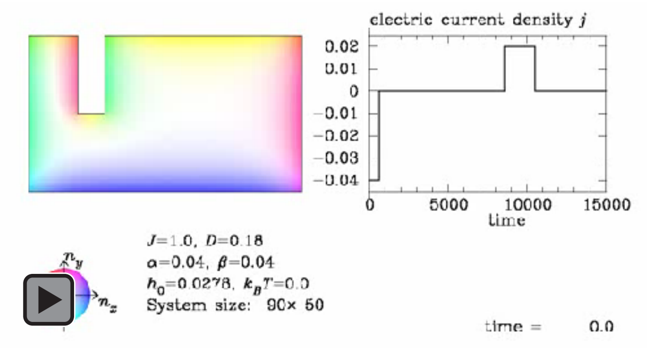


**Movie 6**

Numerical result of Sk motion in the case of Fig.6.

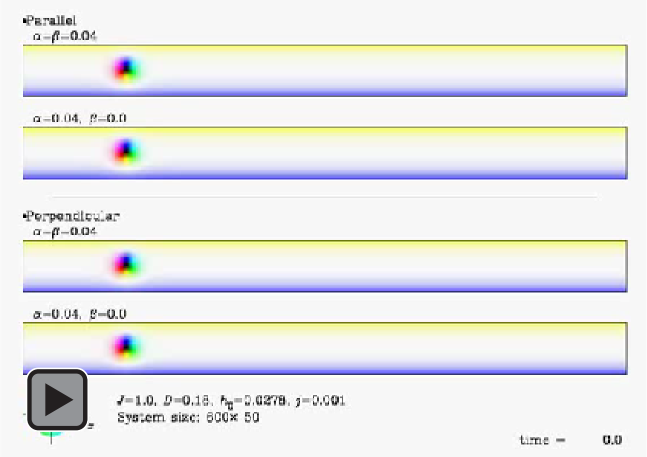

**Movie 7**

Numerical result of the Sk slide-switch memory shown in Fig.7.

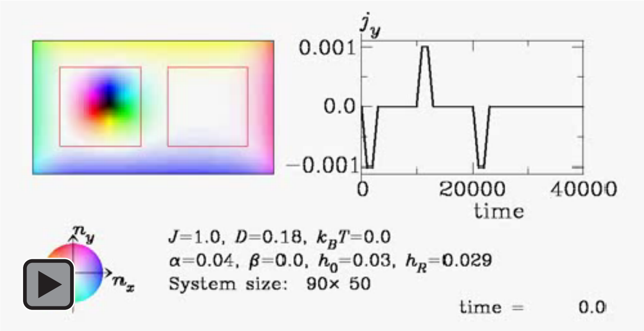


**Movie 8**

Numerical result of the Sk racing-circuit memory shown in Fig.8.

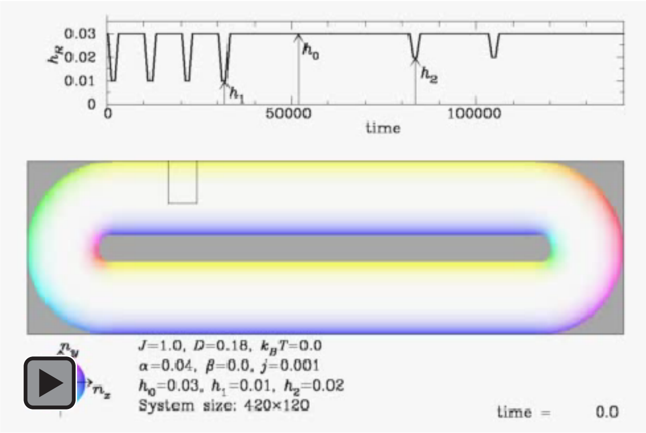


**Movie 9**

Reset procedure of the Sk racing-circuit memory shown in Fig.8.

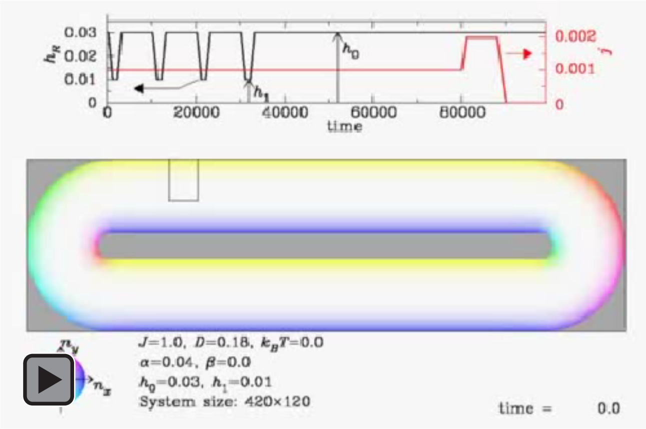

Supplement: Supplementary file 1 [file Supplementary_Informations.pdf]
